# Supplementary material for: Multi-Queues Can Be State-of-the-Art Priority Schedulers
Source: arXiv:2109.00657 source file (2021-09-02)
Supplement: Supplementary file 1 [file appendix_optimizations.tex]

\clearpage

\section{Classic Multi-Queue Optimizations: Implementation Details}

The classic Multi-Queue uses $m$ protected by lock sequential queues and distributes requests among them. When \ins{} comes, it adds the specified task into a random queue, acquiring this queue lock. Similarly, \del{} picks \emph{two} random queues, acquires the corresponding locks, and retrieves the first task from the queue with higher priority. 
Typically, the number of queues $m$ equals the number of worker threads $T$ multiplied by a constant $C$ from the range \texttt{[2..4]}. Therefore, it is likely to take the lock of a random queue without waiting. Since the waiting phase is expensive and it is guaranteed that there are unlocked queues, all the implementations we noticed try to acquire locks and restart the operation from the beginning of the acquisition fails. Figure~\ref{fig:one_lock_in_pop} shows that the non-blocking strategy is better, so we follow the same pattern.

\subsection{Optimistic \del{}}
In the naive Multi-Queue implementation, \del{} acquires both randomly selected queues to choose the better one. Since lock acquisitions are expensive, it would be better to avoid lock acquisitions on making a choice and block only the better queue. 
However, it is possible that between making a choice and acquiring the lock, the situation has changed, so that the better queue becomes worse {---} this way, it leads to a potential work increase. 
Besides, the algorithm should allow reading the highest priority of the queue concurrently with protected by lock modifications.

To read the highest priority in the queue, we maintain a separate \texttt{max} field that stores the task with the highest priority. Listing~\ref{lst:basic_pq} shows the pseudo-code of such a queue protected by a lock. This \texttt{PriorityQueueWithLock} class contains (1) the \texttt{queue} field that stores a sequential $d$-ary heap at line~\ref{line:basic_pq:queue} (usually, $d$ equals 4 since most of CPUs can perform $4$ parallel reads or writes), (2) the \texttt{lock} at line~\ref{line:basic_pq:lock} which is used to protect the sequential queue, and the \texttt{max} field at line~\ref{line:basic_pq:max} that stores the task with the highest priority. In our notation, we use math comparison operations to compare priorities of different tasks. We use this \texttt{PriorityQueueWithLock} as a building block for different Multi-Queue implementations.

\paragraph{\texttt{tryPop()} operation.} 
All Multi-Queue modifications we present in this paper restart the operation when another thread holds the chosen queue lock. Therefore, in \texttt{PriorityQueueWithLock} we implement \texttt{tryPop()} operation that returns a non-null task if the retrieval succeeds, or null if the lock acquisition fails or the queue is empty. 
At first, \texttt{tryPop()} tries to acquire the queue lock at line~\ref{line:basic_pq:tryPop:tryLock}. If the acquisition fails, it immediately returns \texttt{null}. 
After that, the algorithm checks whether the queue is empty and fails in this case, see lines~\ref{line:basic_pq:tryPop:checkMin0}--\ref{line:basic_pq:tryPop:checkMin1} {---} it is possible that between choosing the queue and acquiring the lock, the queue has become empty. 
At last, it retrieves the next task from the sequential heap, replaces it with the current \texttt{max} at lines~\ref{line:basic_pq:tryPop:extract0}--\ref{line:basic_pq:tryPop:extract1} following by releasing the lock at line~\ref{line:basic_pq:tryPop:unlock} and returning the previous \texttt{max} value as the result.

\paragraph{The \texttt{tryPush(..)} operation.} 
Likewise \texttt{tryPop()}, the \texttt{tryPush(..)} operation tries to acquire the lock at first and returns \texttt{false} if fails, see lines~\ref{line:basic_pq:tryPush:tryLock0}--\ref{line:basic_pq:tryPush:tryLock1}. If the lock is taken, it adds the specified task into the sequential queue at line~\ref{line:basic_pq:tryPush:addtasks}, updates the \texttt{max} field at lines~\ref{line:basic_pq:tryPush:updateMax0}--\ref{line:basic_pq:tryPush:updateMax0}, releases the lock at line~\ref{line:basic_pq:tryPush:unlock}, and successfully completes.

\begin{lstlisting}[
label={lst:basic_pq}, 
caption={Sequential priority queue protected by lock. We use this queue as a building block for our practical Multi-Queue implementations.}
]
class PriorityQueueWithLock<E> {
 val queue = Heap<E>() // fast sequential d-ary heap #\label{line:basic_pq:queue}#
 val lock = Lock() // mutex to guard the heap #\label{line:basic_pq:lock}#
 // The task with the highest priority
 // or null if the queue is empty
 var max: E? = null #\label{line:basic_pq:max}#
  
 // Tries to acquire the lock and retrieve the highest
 // priority task. Returns `null` on failure.
 fun tryPop(): E? {
 #\indentrule#  if !mutex.tryLock(): // try to acquire the lock #\label{line:basic_pq:tryPop:tryLock}#
 #\indentrule#  #\indentrule#  return null // the lock is not acquired, fail
 #\indentrule#  if max == null: // is the queue empty? #\label{line:basic_pq:tryPop:checkMin0}#
 #\indentrule#  #\indentrule#  mutex.unlock() 
 #\indentrule#  #\indentrule#  return null // the queue is empty, fail #\label{line:basic_pq:tryPop:checkMin1}#
 #\indentrule#  // Replace `max` with the one from the queue
 #\indentrule#  result := max #\label{line:basic_pq:tryPop:extract0}#
 #\indentrule#  max = queue.extractMax()  #\label{line:basic_pq:tryPop:extract1}#
 #\indentrule#  // Release the lock and return the result  
 #\indentrule#  lock.unlock() #\label{line:basic_pq:tryPop:unlock}#
 #\indentrule#  return result
 }
  
  // Tries to insert the specified task
 fun tryPush(task: E): Bool {
 #\indentrule#  if !lock.tryLock(): // try to acquire the lock  #\label{line:basic_pq:tryPush:tryLock0}#
 #\indentrule#  #\indentrule#  return false // the lock is not acquired, fail #\label{line:basic_pq:tryPush:tryLock1}#
 #\indentrule#  queue.add(task) // add the task to the queue #\label{line:basic_pq:tryPush:addtasks}#
 #\indentrule#  if max < queue.peekMax(): // update `max` if needed #\label{line:basic_pq:tryPush:updateMax0}#
 #\indentrule#  #\indentrule#  queue.add(max)
 #\indentrule#  #\indentrule#  max = queue.extractMax() #\label{line:basic_pq:tryPush:updateMax1}#
 #\indentrule#  lock.unlock() // release the lock #\label{line:basic_pq:tryPush:unlock}#
 #\indentrule#  return true   // and complete successfully
 }
}
\end{lstlisting}
\nk{Pseudo-Code: do not store the max priority task separately, store the priority instead}

\paragraph{Multi-Queue Implementation.}
Our Multi-Queue consists of $K$ \texttt{PriorityQueueWithLock} queues defined at line~\ref{line:basic_mq:queues}. The \ins{} operation is straightforward {---} it chooses a random queue at line~\ref{line:basic_mq:push:rand} and tries to push the task into it at line~\ref{line:basic_mq:push:tryPush}, restarting the operation on failure. The \del{} operation chooses two random queues at lines~\ref{line:basic_mq:pop:rand0}--\ref{line:basic_mq:pop:rand1} and tries to retrieve the task from the better one at lines~\ref{line:basic_mq:pop:tryPopBest0}--\ref{line:basic_mq:pop:tryPopBest1}. For simplicity, our \del{} implementation returns \texttt{null} on failure, even when the Multi-Queue contains tasks. One can maintain the number of non-empty queues and re-start the operation if it is greater than zero. However, the Galois framework that we use for experiments allows such implementation, so we find this simplified version already practical and simpler for understanding. Nevertheless, we discuss how to make this Multi-Queue linearizable in Section~\ref{sec:blocking_mq}.

\begin{lstlisting}[
label={lst:basic_mq}, 
caption={Multi-Queue implementation on the top of \text{PriorityQueueWithLock} that chooses the better queue in \del{} in a non-blocking way.}
]
class MultiQueue<E> {
 val queues = PriorityQueueWithLock<E>[C * T] #\label{line:basic_mq:queues}#
 
 fun push(task: E) = while(true) {
 #\indentrule#  q := random(0, queues.size) #\label{line:basic_mq:push:rand}#
 #\indentrule#  if queues[q].tryPush(task): return #\label{line:basic_mq:push:tryPush}#
 }
 
 fun pop(): E? {
 #\indentrule#  i1, i2 := distinctRandom(0, queues.size) #\label{line:basic_mq:pop:rand0}#
 #\indentrule#  q1 := queues[i1]; q2 := queues[i2] #\label{line:basic_mq:pop:rand1}#
 #\indentrule#  q := q1.max > q2.max ? q1 : q2  #\label{line:basic_mq:pop:tryPopBest0}#
 #\indentrule#  return q.tryPop()   #\label{line:basic_mq:pop:tryPopBest1}#
 }
}
\end{lstlisting}

\paragraph{Experiments.}
Figure~\ref{fig:one_lock_in_pop} shows ... 
\nk{We need an experiment that shows that the time decreases but the total work stays (almost) the same}

\subsection{Buffering}
Listing~\ref{lst:mq_batching} presents a Multi-Queue modification with the buffering optimization for both \ins{} and \del{}. At first, thread-local buffers for these operations are added at lines~\ref{line:mq_batching:pushBuffer}~and~\ref{line:mq_batching:popBuffer} correspondingly. The \ins{} logic is straightforward {---} the algorithm adds the specified task into the buffer at line~\ref{line:mq_batching:push:add} and flushes this buffer to a random queue at line~\ref{line:mq_batching:push:flush}. The \texttt{flushPushBuffer} code is presented at lines~\ref{line:mq_batching:flushPushBuffer:start}--~\ref{line:mq_batching:flushPushBuffer:end} and works similarly to \ins{} operation in the classic Multi-Queue {---} it chooses a random queue and tries to add all buffer tasks via \texttt{tryPush(..)} (we now assume that \texttt{tryPush(..)} can take a list of tasks to be inserted), restarting the operation on failure.

The \del{} operation retrieves multiple tasks into \texttt{popBuffer} and uses it to take new tasks, re-filling the buffer when it becomes empty. The corresponding logic is presented at lines~\ref{line:mq_batching:pop:start}--\ref{line:mq_batching:pop:end}.
When the buffer is empty, the operation tries to refill it via the \texttt{tryFillPopBuffer()}, which works similarly to \del{} in the classic Multi-Queue algorithm. However, the refiling procedure can fail if non-empty queues are not found. In this case, we try to fill \texttt{popBuffer} with the highest priority tasks in \texttt{pushBuffer} at lines~\ref{}--\ref{}. At the end, we either return the first task in \texttt{popBuffer} or \texttt{null} if it is empty, see lines~\ref{}--\ref{}.

\nk{tryFillPopBuffer is subject to change}

\begin{lstlisting}[
label={lst:mq_batching}, 
caption={Multi-Queue implementation with the batching heuristic that retrieves multiple tasks at once and maintains a buffer of tasks to be put, flushing it when is becomes full.}
]
class BatchingMultiQueue<T> {
 val queues = PriorityQueueWithLock<T>[C * threads] 
 threadlocal val pushBuffer = Buffer<T>(PUSH_SIZE) #\label{line:mq_batching:pushBuffer}#
 threadlocal val popBuffer = Buffer<T>(POP_SIZE) #\label{line:mq_batching:popBuffer}#

 fun push(task: T) {
 #\indentrule#  // Add the task to the buffer
 #\indentrule#  pushBuffer.add(task) #\label{line:mq_batching:push:add}#
 #\indentrule#  // Flush the buffer if it has become full
 #\indentrule#  if pushBuffer.isFull(): flushPushBuffer() #\label{line:mq_batching:push:flush}#
 }

 fun flushPushBuffer() = while (true) { #\label{line:mq_batching:flushPushBuffer:start}#
 #\indentrule#  // Try to add the buffer tasks to a random queue
 #\indentrule#  q := random(0, queues.size())
 #\indentrule#  if queues[q].tryPush(pushBuffer): 
 #\indentrule#  #\indentrule#  pushBuffer.clear() 
 #\indentrule#  #\indentrule#  return
 } #\label{line:mq_batching:flushPushBuffer:end}#

 fun pop(): T? { #\label{line:mq_batching:pop:start}#
 #\indentrule#  // Fill in popBuffer if it is empty.
 #\indentrule#  if popBuffer.isEmpty():
 #\indentrule#  #\indentrule#  tryFillPopBuffer()
 #\indentrule#  // Return the first task from the buffer
 #\indentrule#  // or `null` if it is still empty
 #\indentrule#  if popBuffer.isNotEmpty():
 #\indentrule#  #\indentrule#  return popBuffer.removeFirst()
 #\indentrule#  return null
 } #\label{line:mq_batching:pop:end}#

 fun tryFillPopBuffer() {
 #\indentrule#  i1, i2 := distinctRandom(0, queues.size)
 #\indentrule#  q1 := queues[i1]; q2 := queues[i2]
 #\indentrule#  q := q1.max > q2.max ? q1 : q2
 #\indentrule#  // Try to retrieve the task to put into the buffer
 #\indentrule#  tasks := q.tryPop(POP_BUFFER_CAPACITY)
 #\indentrule#  if tasks != null:
 #\indentrule#  #\indentrule#  // The retrieval was successful, fill the buffer
 #\indentrule#  #\indentrule#  popBuffer.fill(tasks)
 #\indentrule#  else: 
 #\indentrule#  #\indentrule#  // Try to fill with the tasks from `pushBuffer`
 #\indentrule#  #\indentrule#  popBuffer.fillFrom(pushBuffer)
 }
}
\end{lstlisting}

\subsection{Local Queues}
Listing~\ref{listing:mq_local} presents the pseudo-code with the local queues heuristic. In contrast to the previous algorithm, we implement the \ins{} operation that takes a list of nodes. Consider an iterative algorithm like the classic for the single-shortest path by Dijkstra. On each step, it relaxes multiple edges and, thus, adds multiple nodes to the queue. Since with the local queues heuristic a sequence of \ins{} invocations manipulate with the same queue, it is better to acquire the queue lock at once for multiple tasks. To guarantee fairness, we do not simply push the whole list to the local queue but split it into batches simulating local queue changes to determine the batch sizes {---} the corresponding code is sown at lines~\ref{line:mq_local:push_batch0}--\ref{line:mq_local:push_batch1}.

When the tasks are split into batches, the algorithm pushes each batch to the same queue via \texttt{pushBatch(..)} function at line~\ref{line:mq_local:push:pushBatch}, updating the local queue after each batch except for the last one, see lines~\ref{line:mq_local:push:updateLocalQ0}--\ref{line:mq_local:push:updateLocalQ1}.
The \texttt{pushBatch(..)} operation tries to put all the tasks into the local queue. However, if the insertion fails due to unsuccessful lock acquisition, the algorithm chooses a new local queue to make progress at line~\ref{line:mq_local:pushBatch:newLocal}. 

The \del{} operation is listed at lines~\ref{}--\ref{} and essentially changes the local queue if needed at lines~\ref{}--\ref{} and tries to retrieve an task from it at line~\ref{}. If the retrieval fails, the local queue is either empty, or another thread holds the lock. Therefore, the algorithm chooses a new local queue at line~\ref{}. To choose a new local queue, the algorithm takes two random ones and selects the better one, see lines~\ref{}--\ref{}.

\begin{lstlisting}[label={listing:mq_local}, 
caption={
Multi-Queue implementation with the local queues for \ins{} and \del{} heuristic. These local queues change with the specified probability or when they are found empty or locked.
}
]
class LocalQueuesMultiQueue<T> {
 val queues: PriorityQueueWithLock<T>[C * threads]
 threadlocal var pushLocalQ: Int // local queue for push
 threadlocal var popLocalQ:  Int // local queue for pop
 
 fun push(tasks: List<T>) {
 #\indentrule#  // We split tasks into batches, so we can acquire
 #\indentrule#  // a queue lock at once for multiple tasks
 #\indentrule#  batches: List<List<T>> := listOf(emptyList()) #\label{line:mq_local:push_batch0}#
 #\indentrule#  for (task in tasks):
 #\indentrule#  #\indentrule#  // Count batch sizes with ChangeQPush probability
 #\indentrule#  #\indentrule#  with ChangeQPush probability {
 #\indentrule#  #\indentrule#  #\indentrule#  // Current batch is done, creating the next one
 #\indentrule#  #\indentrule#  #\indentrule#  batches.add(emptyList()) // create a new batch
 #\indentrule#  #\indentrule#  }
 #\indentrule#  #\indentrule#  batches.last().add(task) #\label{line:mq_local:push_batch1}#
 #\indentrule#  for (batch in batches):
 #\indentrule#  #\indentrule#  pushBatch(batch) #\label{line:mq_local:push:pushBatch}#
 #\indentrule#  #\indentrule#  // Change the local queue if there are more batches
 #\indentrule#  #\indentrule#  if batch != batches.last(): #\label{line:mq_local:push:updateLocalQ0}#
 #\indentrule#  #\indentrule#  #\indentrule#  pushLocalQ := random(0, queues.size) #\label{line:mq_local:push:updateLocalQ1}#
 }

 // Inserts the specified tasks into a single queue.
 fun pushBatch(tasks: List<T>) {
 #\indentrule#  // Try to insert the tasks into the local queue 
 #\indentrule#  // and choose a new until the attempt succeeds.
 #\indentrule#  while !queues[pushLocalQ].tryPush(tasks): 
 #\indentrule#  #\indentrule#  pushLocalQ = random(0, queues.size()) #\label{line:mq_local:pushBatch:newLocal}#
 }

 fun pop(): T? {
 #\indentrule#  // Change the local queue with ChangeQPop probability
 #\indentrule#  with ChangeQPop probability {
 #\indentrule#  #\indentrule#  chooseNewPopLocalQueue()
 #\indentrule#  }
 #\indentrule#  // Try to retrieve a task from the local queue
 #\indentrule#  result := queue[popLocalQ].tryPop()
 #\indentrule#  // Was the retrieval successful?
 #\indentrule#  if result != null: return result
 #\indentrule#  // Change the local queue for the next call
 #\indentrule#  chooseNewPopLocalQueue()
 #\indentrule#  return null
 }
 
 fun chooseNewPopLocalQueue() {
 #\indentrule#  i1, i2 := distinctRandom(0, queues.size)
 #\indentrule#  popLocalQ = queues[i1].max > queues[i2].max ? i1 : i2
 }
}
\end{lstlisting}
