# Supplementary material for: Multi-Queues Can Be State-of-the-Art Priority Schedulers
Source: arXiv:2109.00657 source file (2021-09-02)
Supplement: Supplementary file 2 [file appendix_other_schedulers.tex]

\clearpage
\onecolumn
\section{Approaches for Priority Scheduling}\label{appendix:mq_experiment}

!!!!!!!!!!!!!!!! FEEL FREE TO REMOVE THAT :)

\paragraph{Ordered By Integer Metric (OBIM)~\cite{Nguyen13,PMOD}} The data structure consists of concurrent bags holding pending tasks, each bag corresponds to one priority level (for instance, a priority level $p$ can contain all the tasks with priority $p$). The bags are designed in machine-topology-aware way, including containing fixed-size buffers per core to reduce cache coherence traffic. Once a buffer is filled, the tasks become available for other cores.

The fundamental pillar of the scheduler is the \textit{global map} holding priority-bag pairs, which is read and written by all threads. To reduce the load, the contents of the map are cached by each thread in a \textit{local map}. The design is presented on Figure~\ref{fig:obim:maps}.

\texttt{insert(p, task)} searches for a bag with the priority $p$ in the local map and pushes the task into the bag. If the bag is not cached, a thread synchronizes with the global map, creating a new bag if needed.

\texttt{delete()} traverses the local map in priority order and selects the first non-empty bag.  After that, sequential \texttt{delete()} operations retrieve tasks from the bag until it is empty. If a non-empty bag is not found, the thread synchronizes with the global map, updates its cache and tries again.

As having too few tasks per priority increases map traversal time and communication between threads, most benchmarks are parameterized with \obimdel{}, which determines priority levels as follows: $PL_M = \{task \mid p >> \Delta = M\}$, where $>>$ denotes bitwise right shift operator, $p$ is the priority of the task.

\paragraph{Priority Merging On Demand (PMOD).~\cite{PMOD}} PMOD adopts the approach of OBIM, making the scheduler adaptive. Instead of using a manual parameter \obimdel{}, PMOD dynamically identifies whether the number of priority levels is insufficient or excessive and changes it at runtime. 

\paragraph{Random Enqueue Local Dequeue (RELD).} The data structure consists of $T$ concurrent priority queues, where $T$ is the number of threads. Each priority queue is associated with a thread. 
\texttt{insert(p, task)} pushes the task into a random queue.
\texttt{delete()} retrieves a task from the associated queue, blocking if the queue is empty.

\paragraph{SprayList.~\cite{SprayList}} The SprayList uses a lock-free skip list~\cite{Fomitchev2004}, which stores pending tasks in priority order.
\texttt{insert(p, task)} adds the task into the skip list.
\texttt{delete()} extracts a task from the skip list, emulating a uniform choice among the elements with the highest priority.
